# Supplementary material for: Who is More Bayesian: Humans or ChatGPT?
Source: arXiv:2504.10636 source file (2025-04-14)
Supplement: Supplementary file 1 [file appendix_comparing_estimates_humans_gpts.tex]

\section*{Concise Description of the Four-Parameter Structural-Logit Model}

\noindent
\textbf{Below is a concise, step-by-step description of the four-parameter structural-logit model they use:}

\begin{enumerate}
\item \textbf{Setup}
  \begin{itemize}
    \item There are two bingo cages (A and B) with known probabilities of drawing a certain type of ball (e.g., ``red''), denoted \((p_A, p_B)\).
    \item A prior probability \(\pi\) governs the chance that cage~A (vs.~B) was chosen.
    \item From the chosen cage, \(D\) balls are drawn (with replacement), and \(d\) of them are of the ``marked'' type.
  \end{itemize}

\item \textbf{Log-Prior-Odds and Log-Likelihood-Ratio}
  \[
     \text{LPR}(\pi) \;=\; \ln\!\Bigl(\tfrac{\pi}{\,1-\pi\,}\Bigr),
     \quad
     \text{LLR}(d; p_A, p_B, D) \;=\; \ln\!\Bigl(\tfrac{\,f(d \mid p_A, D\,)}{\,f(d \mid p_B, D\,}\Bigr),
  \]
  where \(f(\cdot\mid p,D)\) is the binomial probability of getting \(d\) marked balls out of \(D\).

\item \textbf{Subjective Posterior Belief}

  A person (or AI agent) may not compute Bayes's rule exactly; instead, their \emph{subjective} posterior \(\Pi_s(A)\) is parameterized by three coefficients \(\beta_0,\beta_1,\beta_2\) plus (potentially) a ``calculation noise'' shock:
  \[
    \ln\!\Bigl(\tfrac{\,\Pi_s(A)\,}{\,1 - \Pi_s(A)\,}\Bigr)
    \;=\;
    \beta_0 + \beta_1 \,\text{LLR} + \beta_2 \,\text{LPR} + \nu.
  \]
  Often \(\nu = 0\) or has small variance, so random ``calculation errors'' can be included.

\item \textbf{Logit Choice}

  Each trial involves choosing either cage~A or B. Let the agent's payoff be \(R>0\) if the choice is correct (0 otherwise). Their decision is modeled with a logistic (softmax) response that depends on \(\Pi_s(A)\). If \(\sigma\) is the scale of ``choice randomness,'' then
  \[
    P(\text{choose A}\mid d,\pi,p_A,p_B)
    \;=\;
    \frac{1}{1 + \exp\!\Bigl(\tfrac{R}{\sigma}\,[1 - 2\,\Pi_s(A)]\Bigr)}.
  \]
  Equivalently, one can say the subject chooses~A whenever
  \[
    R\,\Pi_s(A) - \sigma\,\varepsilon(A) \;>\; R\,[1-\Pi_s(A)] - \sigma\,\varepsilon(B),
  \]
  for \(\varepsilon(\cdot)\) drawn i.i.d.~from a Gumbel (Type-I extreme value) distribution.

\item \textbf{Four Parameters}

  \(\beta_0,\;\beta_1,\;\beta_2\) govern how the subject forms or distorts posterior beliefs from \(\text{LLR}\) and \(\text{LPR}\). 
  \(\sigma>0\) governs how ``noisy'' or random the final cage choice is, given those subjective posterior beliefs.

\end{enumerate}

\noindent
\emph{In short, (i) the model replaces exact Bayesian updating with a logistic-linear ``rule'' in log-prior-odds and log-likelihood-ratios, and (ii) it adds a further logistic ``choice'' layer, controlling random errors when the subject picks a cage. That yields four parameters:}
\[
   \Bigl(\sigma,\;\beta_0,\;\beta_1,\;\beta_2\Bigr).
\]

\vspace{1em}\hrule\vspace{1.5em}

\section*{Context: Structural-Logit Parameters and Perfect Bayesian Benchmarks}

\noindent
\textbf{Below is a brief explanation of what each of the four structural-logit parameters represents and which values characterize a perfect Bayesian in that model.}

\subsection*{1.\quad The Four Parameters}

\paragraph{\(\beta_1\): Weight on the sample evidence}
\begin{itemize}
\item The model uses the \textbf{log-likelihood ratio} (LLR), i.e.\ \(\ln\!\bigl(\tfrac{f(d \mid p_A)}{f(d \mid p_B)}\bigr)\).
\item \(\beta_1\) scales how heavily a person (or AI) weights that sample information.
\item \(\beta_1 > 1\) means the subject \emph{over-reacts} to sample data (\emph{representativeness}).
\item \(\beta_1 < 1\) means the subject \emph{under-reacts} to sample data.
\end{itemize}

\paragraph{\(\beta_2\): Weight on the prior}
\begin{itemize}
\item The model also uses the \textbf{log-prior-odds} (LPR), i.e.\ \(\ln\!\bigl(\tfrac{\pi}{\,1-\pi\,}\bigr)\).
\item \(\beta_2\) is how strongly the subject incorporates prior information.
\item \(\beta_2 > 1\) indicates \emph{overweighting} the prior (\emph{conservatism}).
\item \(\beta_2 < 1\) indicates \emph{underweighting} the prior.
\end{itemize}

\paragraph{\(\beta_0\): Overall bias or baseline shift}
\begin{itemize}
\item This is a constant term added into the log-odds for one cage vs.\ the other.
\item \(\beta_0 > 0\) means systematically favoring Cage~A even if sample and prior are neutral.
\item \(\beta_0 < 0\) means a bias in favor of Cage~B.
\end{itemize}

\paragraph{\(\sigma\): Decision ``noise''}
\begin{itemize}
\item After forming a \emph{subjective} posterior, a subject can still make random (``tremble'') errors.
\item A smaller \(\sigma\) means more deterministic, all-or-nothing choice.
\item A larger \(\sigma\) means significant randomness, effectively more guessing.
\end{itemize}

\subsection*{2.\quad Perfect Bayesian Benchmarks}

\paragraph{Exact Bayes Rule (no misweighting)}
\[
  \beta_0 = 0,\quad \beta_1 = 1,\quad \beta_2 = 1.
\]
No constant bias, and both sample likelihood and prior are correctly weighted.

\paragraph{No Decision Noise (purely deterministic)}
\[
  \sigma = 0.
\]
Then the agent picks whichever cage has the higher posterior probability with certainty.

\noindent
Hence, a \emph{perfectly efficient Bayesian} has:
\[
  (\sigma,\;\beta_0,\;\beta_1,\;\beta_2) \;=\; (0,\,0,\,1,\,1),
\]
yielding purely correct classification in every trial.

\vspace{1.5em}\hrule\vspace{1em}

\section*{Summary of GPT--3.5, GPT--4, and GPT--4o Estimates}

Below is a \emph{brief summary} of the four-parameter structural-logit model estimates
\(\bigl(\sigma,\beta_0,\beta_1,\beta_2\bigr)\) for \textbf{GPT--3.5}, \textbf{GPT--4}, and \textbf{GPT--4o}.
Recall:
\begin{itemize}
\item ``Perfect Bayesian'': \(\beta_0=0,\;\beta_1=1,\;\beta_2=1,\;\sigma=0.\)
\item ``Noisy Bayesian'': allows \(\sigma>0\), but still keeps \(\beta_0=0\) and \(\beta_1=\beta_2=1.\)
\end{itemize}

\subsection*{GPT--4o}

\paragraph{Single Type (100\% of Sample)}\mbox{}

\[
  \hat\sigma \approx 0,\quad 
  \hat\beta_0 \approx 0,\quad
  \hat\beta_1 \approx 0,\quad 
  \hat\beta_2 \approx 0.
\]
\begin{itemize}
\item Statistical tests do \emph{not} reject the perfect or noisy Bayesian hypotheses (p\(\approx 1\)).
\item Conclusion: \textbf{GPT--4o} is essentially a (noiseless) \emph{perfect Bayesian}.
\end{itemize}

\subsection*{GPT--4}

\paragraph{Single Type (100\% of Sample)}\mbox{}

\[
  \hat\sigma \approx 0.00,\quad
  \hat\beta_0,\;\hat\beta_1,\;\hat\beta_2 \approx 0,
\]
but a likelihood-ratio test \emph{rejects} the noisy-Bayesian hypothesis \(\beta_0=0,\;\beta_1=1,\;\beta_2=1\) at
\(\mathrm{p}\approx10^{-37}\).
\begin{itemize}
\item Conclusion: GPT--4 is numerically ``almost Bayesian'' but statistically not on the Bayesian hyperplane
      in the pooled data. It's better than GPT--3.5 but not at GPT--4o's near-perfect level.
\end{itemize}

\subsection*{GPT--3.5}

\paragraph{Two Types (42.2\% vs.\ 57.8\%)}\mbox{}

\[
\begin{aligned}
\text{Type~1 (42\%)}\colon\; &(\sigma,\beta_0,\beta_1,\beta_2)\approx(0.494,\;98.25,\;-141.3,\;-57.75),\\
\text{Type~2 (58\%)}\colon\; &(\sigma,\beta_0,\beta_1,\beta_2)\approx(0.242,\;0.081,\;-0.630,\;-0.100).
\end{aligned}
\]
\begin{itemize}
\item Both types deviate strongly from \((\beta_1=1,\;\beta_2=1)\).
\item Frequently ignoring or reversing priors, nowhere near Bayesian weighting.
\end{itemize}

\subsection*{Overall Takeaway}
\begin{enumerate}
\item \textbf{GPT--4o} is effectively perfect Bayesian: no rejection of \((0,\,0,\,1,\,1)\).
\item \textbf{GPT--4} is close numerically but \emph{fails} the Bayesian hyperplane test (p\(\approx 10^{-37}\)).
\item \textbf{GPT--3.5} splits into two subgroups, both of which are far from any Bayesian weighting.
\end{enumerate}
