# Supplementary material for: Who is More Bayesian: Humans or ChatGPT?
Source: arXiv:2504.10636 source file (2025-04-14)
Supplement: Supplementary file 2 [file appendix_data.tex]

\section{Appendix: Data Collection and GPT Models}

Data collection from OpenAI's ChatGPT models was facilitated through their dedicated API, enabling us to query multiple models and store their responses systematically. We created a grid of hyperparameters (priors, temperature, etc.) that would define the complete prompt, pinged Open AI, and collected the full-text response from which both the AB response and probability value (if applicable) were extracted and stored in a single file.

\subsection*{A Brief History of LLMs}

A brief history of the GPT models can be found in Kalyan, K. S. (2023) and can be summarized in the figure below. Until 2014, text-to-text tasks like translation primarily used autoregressive models like RNN/LSTMs. The central problem was remembering the context in longer sentences. This was solved by the transformer's attention mechanism, which parses sentences as a whole (instead of sequentially) and uses self-attention (the whole sentence tells you which words to pay attention to when translating a word). 

The following models, BERT, GPT, and GPT-2, essentially followed a two-step protocol: (1) a general pre-training step on a text corpus to predict masked words and (2) a supervised fine-tuning step for the specific downstream task (translation, summarization, question answering). A typical strategy was to stack transformers on top of each other to improve performance. 

It turns out that scaling up in model depth, data size, and training length does not show decreasing returns. This led to the first large language model, the GPT3, a 175 billion parameter model stored in 350GB, which is a general-purpose zero-shot learner that could finish any prompt it was provided (translation, summarization, question-answering, poetry). Unlike the previous era, fine-tuning is only done here to structure how the response is provided. 

\begin{figure}[h]
    \centering
    \includegraphics[width=0.8\linewidth]{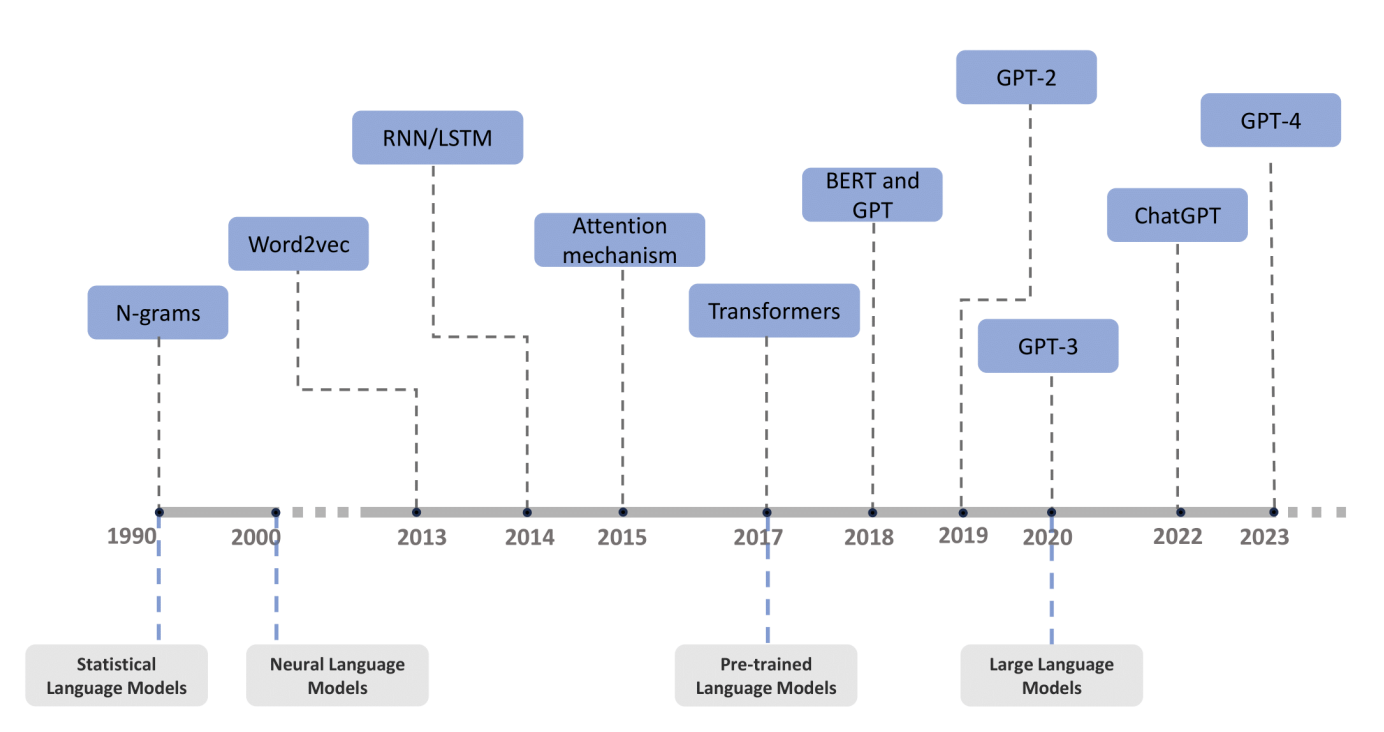}
    %\caption{}
    \label{fig:enter-label}
\end{figure}

\subsection*{Open AI's Models Used in the Study}

We utilized the following GPT models in our experiments:

\begin{itemize}
    \item GPT-3.5-turbo: Released in November 2023, this model is the last and final iteration of the GPT3.5 series. This model is not in active use, having been deprecated in favor of GPT-4o-mini as the "lightweight" AI. This model is optimized for speed and affordability and is suitable for simple text-processing tasks. At its core is the Davinci" base model, which has 175 billion parameters. This base model was improved via instruction training and reinforcement-learning-based human feedback to yield GPT3.5. Further optimizations for speed and cost gave rise to GPT-3.5-Turbo. It is a fast, inexpensive model for functions like fiction writing, translation, summarization, and chatbots and cannot do deep reasoning.
    
    \item GPT-4 and GPT-4-turbo: Released in April 2024, the GPT4 improves over GPT3 through the addition of a larger context window (to process longer text), multimodal capabilities (image, pdf input), plugins that allow it to do programming and search web, more safety features and improved coding abilities. The Turbo version of GPT-4 is an optimized version that increased the speed of execution and overcame some issues of "laziness" in GPT4 where the model would not to do longer tasks. It was released in June 2024, with an even larger context window of 128,000 tokens.
    
    \item GPT-4o: This is OpenAI's current high-intelligence flagship model for complex, multi-step tasks, released on August 6, 2024. GPT-4o is at least as good at reasoning as GPT-4-Turbo and is faster and cheaper. It is designed for tasks requiring advanced reasoning and can handle larger context windows of 128,000 tokens with up to 16,384 output tokens. It is multimodal, accepting text and image inputs, and optimized for structured outputs.
    
    \item GPT-4o-mini: A smaller, more affordable version of GPT-4o designed for fast, lightweight tasks, released on July 18, 2024. It maintains a context window of 128,000 tokens and supports up to 16,384 output tokens. GPT-4o-mini balances performance and efficiency, making it suitable for applications requiring quicker responses without significantly losing reasoning capabilities. It replaced GPT-3.5-Turbo as the lightweight AI. 
\end{itemize}

These models represent a spectrum of capabilities within the GPT family, spanning almost 2 years of continuous development. When this paper was written, the o1-preview and o1-mini models did not have any API functionality. 

\subsection*{Base Prompt and Settings}

The baseline prompt presented to the models described a simple question that involved Bayesian reasoning. The prompt is kept as close to the original formulation as possible:

\begin{quote}
    \textit{There are two bingo cages, Cage A and Cage B. Cage A has 4 red balls and 2 blue balls, and Cage B has 3 red balls and 3 blue balls. A total of \textbf{6} balls will be drawn from one of the cages at random, with replacement after each ball is drawn. One of the two cages from which the 6 balls will be drawn is also randomly selected, and the probability Cage A is selected is \textbf{0.50} and the probability Cage B is selected is \textbf{0.50}. You do not see or know in advance which cage is used to draw the sample of 6 balls. The sample drawn from the selected cage has \textbf{3} red balls and \textbf{3} blue balls.}
\end{quote}

The experiments presented each model with reasoning tasks framed within a grid of base settings. Each model (e.g., GPT4o) was deemed similar to a "college," and multiple trials were taken from "students." Each student was assigned a unique temperature value. Each student did not remember previous questions, since the API did not allow for real-time prompting (so no learning effects).    Key parameters included:

\begin{itemize}
    \item Student, Temperature: Values ranged from 0.5 to 0.9, around the default of 0.7, in a fine grid created by number of students.
    \item Priors: Values ranged from 0.0 to 1.0, including 0.0, 0.1, 0.33, 0.5, 0.67, 0.9, and 1.0, to represent a wide spectrum of initial beliefs.
    \item Total Draws: Fixed at 6 to maintain consistency across trials and simplify computational complexity.
    \item Number of Red Draws: Varied from 0 to the total number of draws (0 to 6), representing all possible outcomes.
    \item Instructions: Four types of instructions were used to assess different reasoning styles and the impact of prompting on model performance.
\end{itemize}

Temperature settings, a parameter that influences the randomness of the model's output, were adjusted between 0.5 and 0.9 across 30 iterations per model to introduce response variability analogous to that observed in human participants.

\subsection*{Instructions / Designs}

Specific instructions were appended to the baseline prompt depending on the design of the experiment. The four types of instructions were intended to collect responses under four different experimental designs:

\begin{enumerate}
    \item AB\_full\_reasoning: Models were instructed to \textit{break the problem into as many steps as possible}, providing detailed reasoning before clearly indicating the answer at the end as ``Final Answer: A'' or ``Final Answer: B''. This design is similar to the California and Wisconsin experiments, but with ample time to reason it out and think slowly.
    
    \item AB\_no\_reasoning: Models were instructed to \textit{directly provide the choice} based on the information, stating ``Final Answer: A'' or ``Final Answer: B'', without any explanation or additional context. This design is similar to the California and Wisconsin experiments, but it has no time to think.
    
    \item prob\_full\_reasoning: Models were presented with an additional gamble scenario and instructed to \textit{break the problem into as many steps as possible}, providing thorough reasoning before indicating the answer at the end as a probability rounded to two decimals (e.g., ``Final Answer: 0.50''). This design is similar to the Holt and Smith experiments, but with full time to reason and think.
    
    \item prob\_no\_reasoning: Models were instructed to \textit{directly state the probability} to maximize their chance of winning a prize, without any explanation or additional context, clearly indicating the answer as a number rounded to two decimals. This design is similar to the Holt and Smith experiments, but has no time to think.
\end{enumerate}

Including phrases like ``break the problem into as many steps as possible'' nudged towards a chain-of-thought reasoning process. Chain-of-thought reasoning has been shown to improve the performance of GPTs. 

\subsection*{Posterior Computation}

The true posterior probability that the sample was drawn from Cage A was calculated using Bayes' theorem, combining the prior probability, total draws, and number of red draws observed. Let \( P(A) \) be the prior probability that Cage A was selected, and \( P(B) = 1 - P(A) \) be the prior probability that Cage B was selected. The total number of draws \( n \) is fixed at 6, with \( k \) representing the number of red balls drawn. The probability of drawing a red ball from Cage A is \( p_{\text{red}|A} = \frac{4}{6} \), and the probability of drawing a red ball from Cage B is \( p_{\text{red}|B} = \frac{3}{6} \).

Using the binomial probability, the likelihood of observing \( k \) red balls from Cage A is calculated as:

\[
L(A) = \binom{n}{k} (p_{\text{red}|A})^k (1 - p_{\text{red}|A})^{n - k}
\]

Similarly, the likelihood for Cage B is:

\[
L(B) = \binom{n}{k} (p_{\text{red}|B})^k (1 - p_{\text{red}|B})^{n - k}
\]

The posterior probability that the sample was drawn from Cage A is then:

\[
P(A \mid \text{data}) = \frac{P(A) \cdot L(A)}{P(A) \cdot L(A) + P(B) \cdot L(B)}
\]

This posterior probability was calculated for each combination of prior \( P(A) \) and the observed number of red draws \( k \), serving as a benchmark for assessing the models' responses. This is the ``correct answer" that a well-reasoned answer would arrive at.

\section*{Algorithm}

\begin{algorithm}[H]
\caption{Data Collection and Processing}
\begin{algorithmic}[1]
    \STATE \textbf{Initialize} OpenAI API using secure API key

    \STATE \textbf{Set parameters:}
    \STATE \quad Models, Priors, Total Draws, Number of Red Draws, Temperature Settings, and Instructions

    \FOR{each combination of Model, Prior, Total Draws, Number of Red Draws, Temperature, and Instruction}
        \STATE Generate prompt using \texttt{generate\_question}
        \STATE Calculate true posterior using \texttt{calculate\_true\_posterior}
        \STATE Send prompt to OpenAI API with error handling
        \STATE Capture response from the API
        
        \IF{Instruction is choice-based}
            \STATE Extract choice using \texttt{extract\_choice}
        \ELSIF{Instruction is probability-based}
            \STATE Extract probability using \texttt{extract\_probability}
        \ENDIF

        \STATE Record metadata and response in CSV file
    \ENDFOR

    \STATE \textbf{Data Processing:}
    \STATE Use regular expressions to parse and extract choice or probability consistently
    \STATE Clip extracted probabilities to [0,1] if necessary

    \STATE \textbf{Posterior Calculation:}
    \STATE Compute true posterior using Bayes' theorem with prior, number of red draws, and total draws as inputs

    \STATE \textbf{Store Data:} Save all processed data with metadata for further analysis
\end{algorithmic}
\end{algorithm}
