# Supplementary material for: Who is More Bayesian: Humans or ChatGPT?
Source: arXiv:2504.10636 source file (2025-04-14)
Supplement: Supplementary file 3 [file appendix_faq.tex]

\section{FAQ}

Q1. Why not just analyze GPT's text explanations directly, instead of treating it as a black box?

We focus on a decision-theoretic approach, judging whether GPT’s final responses align with Bayes’ rule rather than dissecting every chain-of-thought. Textual explanations can be messy or inconsistent, and modeling each arithmetic or logical slip is cumbersome. By treating GPT as a black box, we capture whether it is “as if” Bayesian in its ultimate output, independent of how it arrives there. This aligns with real-world usage, where users generally only see GPT’s final recommendations.

Q2. Aren’t we just testing GPT’s arithmetic rather than its reasoning?

Although Bayesian tasks involve math, they also require weighting priors and likelihoods in a coherent way. In practical settings such as pricing or investment, decision-makers care primarily about whether the model yields rational recommendations. Thus, the core question is whether GPT behaves like a rational agent, not whether it can perform perfect arithmetic at every step.

Q3. How did you collect data from GPT, and what does it look like?

We replicated well-known human-experiment designs that ask, for example, which of two bingo cages likely generated certain draws. We prompted GPT with these questions and recorded its binary choice or reported posterior. A simple flowchart describes each question being posed, GPT producing an answer, and us storing the outcome. This mirrors the procedure used in human trials and allows direct comparison of GPT’s decisions with established human data.

Q4. Could GPT be memorizing these tasks (data leakage), rather than truly reasoning?

Even if GPT has memorized similar problems, the outcome still either matches or deviates from Bayes in consistent ways. We sometimes reword or change the problem context (such as switching from bingo cages to fishing-lake examples) to test whether performance holds. Rapid improvements in newer GPT versions also suggest black-box behavior continues to evolve, indicating more than rote memorization alone.

Q5. What if GPT has already encountered this exact data or tasks?

We can probe GPT’s memory or vary the prompts’ phrasing to see if answers change. Consistent decisions across different wordings suggest GPT is not merely re-spitting memorized solutions. From a decision-theory perspective, the key is whether the final answers align with Bayes—how much stems from training data versus derived reasoning matters less if the conclusion is the same.

Q6. Why not look at GPT’s internal neurons to gauge its logic?

We lack access to proprietary models’ hidden layers, and in any case most users interact with GPT purely via its input-output interface. Our main interest is whether GPT’s decisions align with Bayesian rationality, which is testable through the prompts and final choices. Interpretability at the neuron level is a different research agenda typically addressed by computer scientists.

Q7. Why focus on GPT models only, and not other LLMs like Claude or DeepSeek?

GPT is currently dominant and serves as a clear reference point. However, our econometric testing framework can be applied to any language model, so comparing multiple LLMs is straightforward in principle. As these models evolve, the method of using Bayesian tasks to measure rationality remains valuable for highlighting similarities or differences in their decision behavior.

Q8. If we give GPT more detailed instructions or feedback, could it become fully Bayesian?

We tried various prompt strategies, including chain-of-thought and explicit warnings about the importance of accuracy. While some mistakes decreased, we still observed occasional errors. Multi-round dialogues might reduce errors further, yet some lapses appear persistent. Measuring GPT’s deviation from Bayes in a single-shot setting provides insight into its baseline decision-making performance.

Q9. Why measure deviation from Bayes’ rule, and is it useful for improving AI?

Bayesian updating is a long-established standard in economics and decision theory. Firms deploying GPT in large-scale tasks, such as customer management or pricing, care whether its suggestions align with rational norms. If GPT or weaker variants deviate systematically from Bayes, that may lead to inefficiencies or misguided decisions. Quantifying these biases informs both developers and end-users about potential risks, offering a roadmap for targeted improvements.
