# Supplementary material for: Who is More Bayesian: Humans or ChatGPT?
Source: arXiv:2504.10636 source file (2025-04-14)
Supplement: Supplementary file 4 [file appendix_gpt_vs_bayes.tex]

\section{Appendix: Survey of studies comparing GPTs and Humans}

In this appendix, we consider a large number of studies that directly compare GPTs with humans. In many non-textual logical tasks and reasoning, we find GPT performance comparable to amateurs but not as good as experts. While in more ``textual" tasks, GPTs tend to outperform humans.  

% Increase row height with arraystretch

\begin{singlespace}
\begin{footnotesize}

\begin{longtable}{p{0.9in} p{1.5in} p{1.9in} p{1.9in}}
\caption{Summary of Studies Comparing GPTs with Humans} \label{tab:gpt_vs_humans} \\
\toprule
\textbf{Authors} & \textbf{Question} & \textbf{Data \& Design} & \textbf{Inference} \\
\midrule
\endfirsthead

\multicolumn{4}{c}{{\tablename\ \thetable{} -- continued from previous page}} \\
\toprule
\textbf{Authors} & \textbf{Question} & \textbf{Data \& Design} & \textbf{Inference} \\
\midrule
\endhead

\midrule \multicolumn{4}{r}{{Continued on next page}} \\
\endfoot

\bottomrule
\endlastfoot

\textbf{Frieder et al.\newline (2023)} &
Can ChatGPT solve advanced-level mathematics problems? &
\textbf{Data:} GHOSTS dataset with graduate-level math problems in six sub-datasets; evaluated ChatGPT (Jan 9 and Jan 30, 2023 versions) and GPT-4.\newline
\textbf{Design:} Solving problems from sub-datasets: Grad-Text, Holes-in-Proofs, Olympiad-Problem-Solving, Symbolic-Integration, MATH, and Search-Engine-Aspects. &
\textbf{Inference:} GPT-4 outperformed ChatGPT 3.5 but struggled with complex proofs and advanced computations. Achieved average rating of 4.15 vs.\ ChatGPT's 3.29 on miniGHOSTS. Both models failed on graduate-level and Olympiad problems, often missing critical proof steps or misinterpreting statements. \\

\addlinespace

\textbf{Herbert et al.\newline (2024)} &
Does GPT-4 demonstrate higher creative potential than humans in divergent thinking tasks? &
\textbf{Data:} 151 human participants and matched GPT-4 instances performed Alternative Uses Task (AUT), Consequences Task (CT), and Divergent Associations Task (DAT).\newline
\textbf{Design:} Generate creative uses for common objects, potential outcomes for hypothetical scenarios, and list 10 diverse nouns. &
\textbf{Inference:} GPT-4 outperformed humans in originality and elaboration. In AUT, scored 35\% higher in originality; responses were 4.5 times more detailed. In CT, 42\% higher originality; 7 times more elaboration. In DAT, semantic distances 10\% greater, indicating stronger conceptual variation. \\

\addlinespace

\textbf{Jones and Bergen\newline (2024)} &
Is GPT-4 indistinguishable from humans in conversation during a Turing test? &
\textbf{Data:} 500 participants engaged in 5-minute conversations with either a human or AI models (GPT-4, GPT-3.5, ELIZA); participants judged their interlocutor's humanity.\newline
\textbf{Design:} Engage in open-ended conversations and determine if partner is human or AI. &
\textbf{Inference:} GPT-4 achieved 54\% pass rate, higher than GPT-3.5 (50\%) and ELIZA (22\%), but below humans (67\%). Participants couldn't reliably distinguish GPT-4 from humans; judgments based on conversational style rather than factual accuracy. Age negatively correlated with identification accuracy. \\

\addlinespace

\textbf{Li et al.\newline (2024)} &
Can GPT-4 identify themes in qualitative health care data as effectively as human researchers? &
\textbf{Data:} Interviews from 20 patients with adult-acquired buried penis; comparison between GPT-4 and human thematic analysis using Cohen's kappa for agreement.\newline
\textbf{Design:} Analyze interview transcripts to identify key themes and subthemes related to patient experiences. &
\textbf{Inference:} GPT-4 achieved moderate agreement with human-coded themes ($\kappa=0.401$). Identified major themes like "urinary issues" (75\%) and "sexual issues" (80\%), but fewer subthemes. Humans identified more specific issues such as "pain with sex" and "depression" more frequently. \\

\addlinespace

\textbf{Taloni et al.\newline (2023)} &
How does GPT-4 perform compared to humans and GPT-3.5 on ophthalmology multiple-choice questions? &
\textbf{Data:} 1,023 questions from AAO BCSC self-assessment across ten subspecialties and three practice areas; compared accuracy rates among humans, GPT-3.5, and GPT-4.\newline
\textbf{Design:} Answer multiple-choice questions covering topics like Cataract/Anterior Segment, Glaucoma, Diagnostics/Clinics, Medical Treatment, Surgery. &
\textbf{Inference:} GPT-4 achieved 82.4\% accuracy, outperforming humans (75.7\%) and GPT-3.5 (65.9\%). Performed better in Glaucoma and Oculoplastics but struggled with surgery-related questions. Incorrect answers were longer, indicating verbosity when uncertain. \\

\addlinespace

\textbf{Katz et al.\newline (2024)} &
Can GPT-4 achieve physician-level performance on medical board exams? &
\textbf{Data:} Tested GPT-3.5 and GPT-4 on 2022 Israeli board residency exams in five specialties; compared with results from 849 physicians.\newline
\textbf{Design:} Answer exam questions from internal medicine, general surgery, psychiatry, pediatrics, and OB/GYN specialties. &
\textbf{Inference:} GPT-4 passed four out of five specialties, ranking above median physician in psychiatry (74.7th percentile). Performed similarly to median in internal medicine and surgery; lower in pediatrics and OB/GYN. GPT-3.5 failed to pass any specialty. \\

\addlinespace

\textbf{Yan et al.\newline (2024)} &
How does GPT-4's translation quality compare to human translators across languages and domains? &
\textbf{Data:} Texts in language pairs: Chinese-English, Russian-English, Chinese-Hindi; domains include news, technology, biomedical; errors labeled using MQM schema.\newline
\textbf{Design:} Translate texts between language pairs in various domains; translations evaluated by expert annotators. &
\textbf{Inference:} GPT-4 performed comparably to junior translators in total errors but lagged behind medium and senior translators. Better fluency but more accuracy-related errors. Performance decreased in resource-poor languages like Chinese-Hindi. Tended to produce more literal translations. \\

\addlinespace

\textbf{Martínez\newline (2024)} &
Can GPT-4 perform at or above the passing level on the Uniform Bar Examination? &
\textbf{Data:} Evaluated GPT-4's performance on UBE using official NCBE data and compared with attorney performance.\newline
\textbf{Design:} Answer UBE questions, including multiple-choice (MBE) and essay sections (MEE and MPT). &
\textbf{Inference:} GPT-4 ranked in 69th percentile overall; 62nd percentile using NCBE data. Struggled with essay sections, scoring in 48th percentile (42nd percentile with NCBE data). Performed lower compared to licensed attorneys; few-shot prompting improved results. \\

\addlinespace

\textbf{Yeadon et al.\newline (2024)} &
Can GPT-4 perform at the level of university students in a physics coding course? &
\textbf{Data:} 50 student submissions compared with AI-generated submissions (GPT-3.5 and GPT-4) on Python coding assignments in a university physics course.\newline
\textbf{Design:} Complete coding assignments using Python; tasks involved physics problem-solving and data visualization. &
\textbf{Inference:} GPT-4 with prompt engineering scored 81.1\%; students averaged 91.9\%. GPT-3.5 scored between 30.9\% and 48.8\%. AI submissions were distinguishable from human work 85.3\% of the time due to default plotting styles and misalignments. \\

\addlinespace

\textbf{Herbold et al.\newline (2023)} &
Can AI-generated essays match or exceed the quality of human-written essays? &
\textbf{Data:} 270 essays (human and AI-generated) across 90 topics; rated by 111 teachers; linguistic analysis performed to compare text quality and structure.\newline
\textbf{Design:} Write argumentative essays on assigned topics; GPT-3.5 and GPT-4 generated essays using the same prompts as human students. &
\textbf{Inference:} GPT-4 outperformed human essays in most criteria, including logical structure, language mastery, and vocabulary richness. Teachers rated GPT-4's essays about one point higher on a seven-point scale. Noted that AI essays had more complex sentences and nominalizations; humans used more modals and varied argumentation styles. \\

\end{longtable}

\end{footnotesize}
\end{singlespace}

%% Old ChatGPT documents

Next, we extend the human experiments by leveraging the advantages of ChatGPT. There are two key benefits to conducting experiments with ChatGPT. First, ChatGPT experiments are both cost-effective and time-efficient. Unlike human experiments, the costs are minimal, and we can conduct a large number of experiments in a short period. This enables us to gather responses across a wide range of specifications and explore ChatGPT's performance beyond the limits observed in human subjects. Second, unlike human participants, ChatGPT can provide a comprehensive display of its reasoning process in its responses. This allows us to investigate more deeply why ChatGPT may make more or fewer mistakes compared to humans. We describe the extensions we did below and the details of the prompts and implementations are given in the Appendix.

We first expand the range of prior probabilities. In all human experiments, the prior probabilities that the sample is drawn from one cage range from 0.3 to 0.7. However, as discussed in Section XXX, the structural logit model is only identifiable under extreme priors, akin to the special regressor argument presented by \citet{lewbel2019identification}. Therefore, we also conducted ChatGPT experiments with prior probabilities that spanned the entire interval from 0 to 1.

Second, instead of requiring ChatGPT to skip its reasoning process and present only the final answer, we allow it to display its reasoning step by step. This approach enables us to test whether chain-of-thought prompting \citep{wei2022chain} can enhance ChatGPT's performance on this task. By collecting responses at each step of its reasoning process, we can conduct an error analysis to identify the specific step(s) where ChatGPT makes mistakes.

Third, we investigate whether AI subjects are influenced by "framing" and contextual effects. Since training data for large language models consist primarily of human-generated content that reflects behavioral biases \citep{KT1974}, we aim to test whether ChatGPT inherits these biases in this specific task. To do this, we present essentially the same binary classification problem within a different context \textcolor{red}{describe the context here} and ask AI subjects to respond to these variations.

\textcolor{red}{We should list all the desired LLM experiments here. One example: allow for learning effects?}

Table \ref{table_basic_statistics} provides the basic statistics of various ChatGPT experiments. \textcolor{red}{Why do we have different number of subjects in various experiments? Why do we have subjects without making a final choice? Those look very arbitrary! We could delete this Table once we clear these questions.}

\begin{table}[H]
  \centering
  \caption{Basic Experiments in LLMs}
    \begin{tabular}{lcccccc}
    \toprule
    \toprule
    LLMs  & \multicolumn{2}{c}{GPT 3.5} & \multicolumn{2}{c}{GPT 4} & \multicolumn{2}{c}{GPT 4o} \\
    Step-by-step reasoning & NO    & YES   & NO    & YES   & NO    & YES \\
    \midrule
    Num. of subjects & 50    & 30    & 30    & 30    & 50    & 50 \\
    Num. of trials & 77    & 77    & 77    & 77    & 77    & 77 \\
    \% of missing choices & 0     & 0.91  & 0     & 5.5   & 0     & 0.86 \\
    \% of trials without variations & 14.29 & 10.39 & 92.21 & 16.88 & 84.42 & 29.87 \\
    \bottomrule
    \end{tabular}%
  \label{table_basic_statistics}%
\end{table}%

\subsection{Descriptive of ChatGPT Data}

To evaluate the performance of large language models, Table \ref{table_chatGPT_consistent_choices} presents the proportion of trials in which subjects' choices align with Bayes' rule. This table highlights three key patterns. 

First, there is a notable improvement from ChatGPT 3.5 to ChatGPT 4, but the advancement from ChatGPT 4 to ChatGPT 4o is moderate, or even shows a decline. Second, even with the more advanced ChatGPT 4 and ChatGPT 4o, the proportion of choices consistent with Bayes' rule remains lower than that of human subjects. In the California experiment, the proportion of choices consistent with Bayes' rule was 81\%, which is 10\% higher than that of ChatGPT 4. This indicates sub-human performance, contrasting with several previous studies (more citations needed). 

Third, Table \ref{table_chatGPT_consistent_choices} reveals that, when compared to experiments employing step-by-step reasoning (as shown in the second column), directly reporting results without presenting the reasoning process leads to significantly higher rates of choices consistent with Bayes' rule. This finding contradicts the conclusions drawn by \citet{wei2022chain}, who suggested that chain-of-thought reasoning enhances the performance of LLMs. Additionally, Table \ref{table_basic_statistics} indicates that responses from ChatGPT experiments that directly reported results were almost uniform across subjects within a trial.

In our binary classification tasks, directly reporting results outperforms chain-of-thought reasoning and yields more uniform responses for the following reasons. Large language models (LLMs) translate words into tokens and use preceding words in a sentence to predict the next token. When not using step-by-step reasoning, the LLM essentially only needs to predict two tokens: the word "cage" and either "A" or "B." This simplifies the task significantly. 

However, when the entire reasoning process is displayed, LLMs must predict a larger number of tokens, which introduces more variability in their responses. Additionally, during each prediction step, the LLM calculates components of the Bayesian formula, and there is a chance of making errors at each step. As the number of steps increases, the likelihood of accumulating these errors also rises, making it more probable that ChatGPT will reach an incorrect final decision.

\begin{table}[H]
  \centering
  \caption{Shares of Choices Consistent with Bayes' Rule}
    \begin{tabular}{lcc}
    \toprule
    \toprule
          & Directly report (\%) & Step-by-step reasoning (\%) \\
    \midrule
    GPT 3.5 & 45    & 39 \\
    GPT 4 & 71    & 50 \\
    GPT 4o & 67    & 51 \\
    \bottomrule
    \end{tabular}%
  \label{table_chatGPT_consistent_choices}%
\end{table}%

One distinction between human and LLM experiments is that the latter spans a broader range of prior probabilities, including more extreme values. Table \ref{table_chatGPT_consistent_by_priors} compares the choices consistent with Bayes' rule in two subgroups: one consisting of choices from trials with moderate priors between 0.3 and 0.7, similar to the prior specifications in human subjects, and the other consisting of choices from trials with more extreme priors below 0.3 or above 0.7. Surprisingly, the LLM performs significantly worse under more extreme priors. \textcolor{red}{This result suggests that the comparison in Table \ref{table_chatGPT_consistent_choices} may be misleading, as we do not know how humans perform under extreme priors where LLMs exhibit significantly worse performance.}

\begin{table}[H]
  \centering
  \caption{Shares of Choices Consistent with Bayes' Rule, by Ranges of Priors}
    \begin{tabular}{lcccc}
    \toprule
    \toprule
          & \multicolumn{2}{c}{Moderate priors} & \multicolumn{2}{c}{Step-by-step priors} \\
          & Directly report (\%) & Step-by-step (\%) & Directly report (\%) & Step-by-step (\%) \\
    \midrule
    GPT 3.5 & 45    & 39    & 45    & 39 \\
    GPT 4 & 71    & 50    & 71    & 50 \\
    GPT 4o & 67    & 51    & 67    & 51 \\
    \bottomrule
    \end{tabular}%
  \label{table_chatGPT_consistent_by_priors}%
\end{table}%

\subsection{Structural Model Estimation and Comparison with Human Data}

\subsubsection{Binary Classification: Single-type}

To determine whether the AI subjects are Bayesian, we apply the the El-Gamal and Grether's integer cutoff models,\footnote{The implementation of the estimation algorithm for El-Gamal and Grether's integer cutoff models differs slightly from the analysis for human subjects. In the human experiments, there are three possible priors, leading to 512 potential cutoff rules for each subject. In contrast, the ChatGPT experiment considers priors ranging from 0.1 to 0.9, resulting in over 134 million possible cutoff rules. To tackle the curse of dimensionality that arises from the extensive number of priors and their combinations, we employ a nested algorithm for model estimation. In the outer loop, we search for the error rate $\varepsilon$  to maximize the log likelihood function. In the inner loop, we calculate the likelihood for observations with different prior probabilities separately and then sum them to obtain the total likelihood for all observations.} and the structural logit model to the data generated from ChatGPT experiments. Since it is not possible to calculate the log prior ratios when the prior is 0, we restrict our analysis to choices where the priors are strictly between 0 and 1.\footnote{We can calculate the log prior ratios for choices in trials with a prior of 1; however, to maintain symmetry, we exclude these from our estimation sample.}

Table \ref{table_chatGPT_El-Gamal and Grether} presents the estimation results for the El-Gamal and Grether models. The first column displays the perfectly Bayesian cutoffs. For extreme priors, an optimal decision rule would be to consistently choose one cage, regardless of the ball composition in the experimental sample. For instance, a rational subject should always choose Cage B when the prior probability for Cage A is 0.1, while with a prior of 0.9, the selection should consistently be Cage A. As the prior probability increases, the Bayesian cutoff steadily decreases, suggesting that it is optimal for subjects to choose A when they observe a larger range of possible numbers of red balls.

Similar to human subjects, I find that no LLMs are perfectly Bayesian. However, more advanced LLMs are closer to perfectly Bayesian. Estimates indicate that ChatGPT 3.5, when providing direct responses, aligns with Bayesian cutoffs only for four prior probabilities: 0.1, 0.2, 0.6, and 0.8. When using step-by-step reasoning, ChatGPT 3.5 aligns with Bayesian cutoffs at lower prior probabilities but deviates significantly at higher ones. The estimated cutoffs for GPT 4 and 4o are closer to the Bayesian cutoffs. Among nine prior probabilities, GPT 4 using step-by-step reasoning matches Bayesian cutoffs for eight of them, while GPT 4o is consistent with just one fewer. Although GPT 4o performs slightly worse than GPT 4 in relation to the Bayesian cutoffs, GPT 4 shows more noise, as suggested by a larger value of the error rate compared with ChatGPT 4o.

\begin{table}[H]
  \centering
  \caption{ChatGPT: El-Gamal and Grether Integer Cutoff Model}
    \begin{tabular}{lccccccc}
    \toprule
    \toprule
    LLMs  & Bayesian & \multicolumn{2}{c}{GPT 3.5} & \multicolumn{2}{c}{GPT 4} & \multicolumn{2}{c}{GPT 4o} \\
    Step-by-step reasoning &       & NO    & YES   & NO    & YES   & NO    & YES \\
    \midrule
    0.1   & 6     & 6     & 6     & 3     & 6     & 6     & 6 \\
    0.2   & 5     & 5     & 5     & 3     & 5     & 3     & 5 \\
    0.3   & 4     & 3     & 4     & 3     & 5     & 3     & 4 \\
    0.4   & 4     & 3     & 3     & 3     & 4     & 3     & 3 \\
    0.5   & 3     & 2     & 0     & 3     & 3     & 3     & 3 \\
    0.6   & 2     & 2     & [0,1] & 3     & [2,3] & 3     & 2 \\
    0.7   & 2     & 1     & 0     & 3     & 2     & 3     & 1 \\
    0.8   & 1     & 1     & -1    & 3     & 1     & 3     & 1 \\
    0.9   & 0     & 1     & 0     & 3     & 0     & 3     & 0 \\
    Error rate &       & 0.36  & 0.4615 &      & 0.2928 & 0.00749 & 0.1808 \\
          &       &       &       &       &       &       &  \\
    N     &       & 3150  & 1872  & 1890  & 1769  & 3150  & 3120 \\
    Log likelihood &       & -1484.89 & -1011.26 &       & -736.67 & -503.33 & -946.69 \\
    \bottomrule
    \end{tabular}%
  \label{table_chatGPT_El-Gamal and Grether}%
\end{table}%

Table \ref{table_ChatGPT_structural_logit} presents the estimation results for the structural logit model. We also compare the performance of the structural logit model with El-Gamal and Grether's integer cutoff model using Vuong's non-nested test. Consistent with findings from human subjects, the Vuong test indicates that the structural logit model significantly outperforms the El-Gamal and Grether model across all LLMs. \textcolor{red}{We now focus on discussing the estimation results only for ChatGPT with step-by-step reasoning as there are obviously estimation issues when applying the structural logit model to ChatGPT 4 and 4o with direct responses.}

Table \ref{table_ChatGPT_structural_logit} first confirms that no versions of LLMs adhere to Bayes' rule, as the coefficients associated with log likelihood ratios and log prior ratios significantly deviate from -1 \textcolor{red}{(add t-statistics here)}. Leveraging the ability to elicit underlying beliefs from the structural logit model, we find that subjects assign nearly equal weights to both log likelihood ratios and log prior ratios in all LLMs. This indicates that AI subjects value prior information and posterior information equally, contrasting with human subjects, who tend to place more weight on prior information than on posterior information. Similar to the estimation of the El-Gamal and Grether model, we find that more recent LLMs perform better than the original ChatGPT 3.5, \textcolor{red}{as evidenced by the estimated intercepts being closer to zero for the newer models.} 

\begin{table}[H]
  \centering
  \caption{ChatGPT: Structural Logit Model}
    \begin{tabular}{lccccccc}
    \toprule
    \toprule
    LLMs  & Bayesian & \multicolumn{2}{c}{GPT 3.5} & \multicolumn{2}{c}{GPT 4} & \multicolumn{2}{c}{GPT 4o} \\
    Step-by-step reasoning &       & NO    & YES   & NO    & YES   & NO    & YES \\
    \midrule
    $\beta_0$    & 0     & -0.37 & -0.13 & -0.07 & 0.03  & 2.76  & -0.13 \\
          &       & (0.06) & (0.33) & –     & (0.07) & (3.94) & (0.04) \\
    Log likelihood ratio   & -1    & -0.75 & -0.11 & -1.63 & -1.4  & -26.67 & -1.65 \\
          &       & (0.13) & (0.26) & –     & (0.22) & (14.25) & (0.19) \\
    Log prior ratio   & -1    & -0.67 & -0.16 & -0.16 & -1.32 & -2.41 & -1.54 \\
          &       & (0.11) & (0.39) & –     & (0.21) & (1.37) & (0.18) \\
    $\sigma$ &       & 0.27  & 0.08  & 0     & 0.33  & 0.31  & 0.25 \\
          &       & (0.03) & (0.19) & 0.00  & (0.03) & (0.01) & (0.02) \\
          &       &       &       &       &       &       &  \\
    N. observations &       & 3150  & 1872  & 1890  & 1769  & 3150  & 3120 \\
    Log Likelihood  &       & -1373.41 & -922.54 & –     & -669.95 & -547.07 & -806.08 \\
    Vuong test stat  &       & 4.02  & 4.05  & –     & 3.15  & -1.79 & 5.58 \\
    P-value (against EG) &       & 5.92E-05 & 5.16E-05 & –     & 0.0016 & 0.073254 & 2.34E-08 \\
    \bottomrule
    \end{tabular}%
  \label{table_ChatGPT_structural_logit}%
\end{table}%

We then calculate the loss functions and compare them to those obtained from the human subjects. [\textcolor{red}{The results are TBA. Should we also plot the CCPs here?} ] 

\subsubsection{Binary Classification: Multiple-types}

We then investigate whether there are unobserved heterogeneity across AI subjects and try to detect them using the modified EC algorithm with thresholds. [\textcolor{red}{The results are TBA. Then we compare the estimated CCPs with human subjects.} ] 

\subsubsection{Posterior Probabilities}

LLM experiments akin to \citet{HS2009}.

\subsection{Why do ChatGPT perform worse than human beings?}

\textcolor{red}{Do economists care about the answers to this question?}
